# Supplementary material for: Embedding Arithmetic of Multimodal Queries for Image Retrieval
Source: arXiv:2112.03162 source file (2022-10-20)
Supplement: Supplementary file 1 [file supmat.tex]

\clearpage
\appendix

\section{Supplementary Material}
\label{sec:appendix}

\subsection{Transformation score by target}

\begin{figure}[H]
    \centering
    \includegraphics[width=\linewidth]{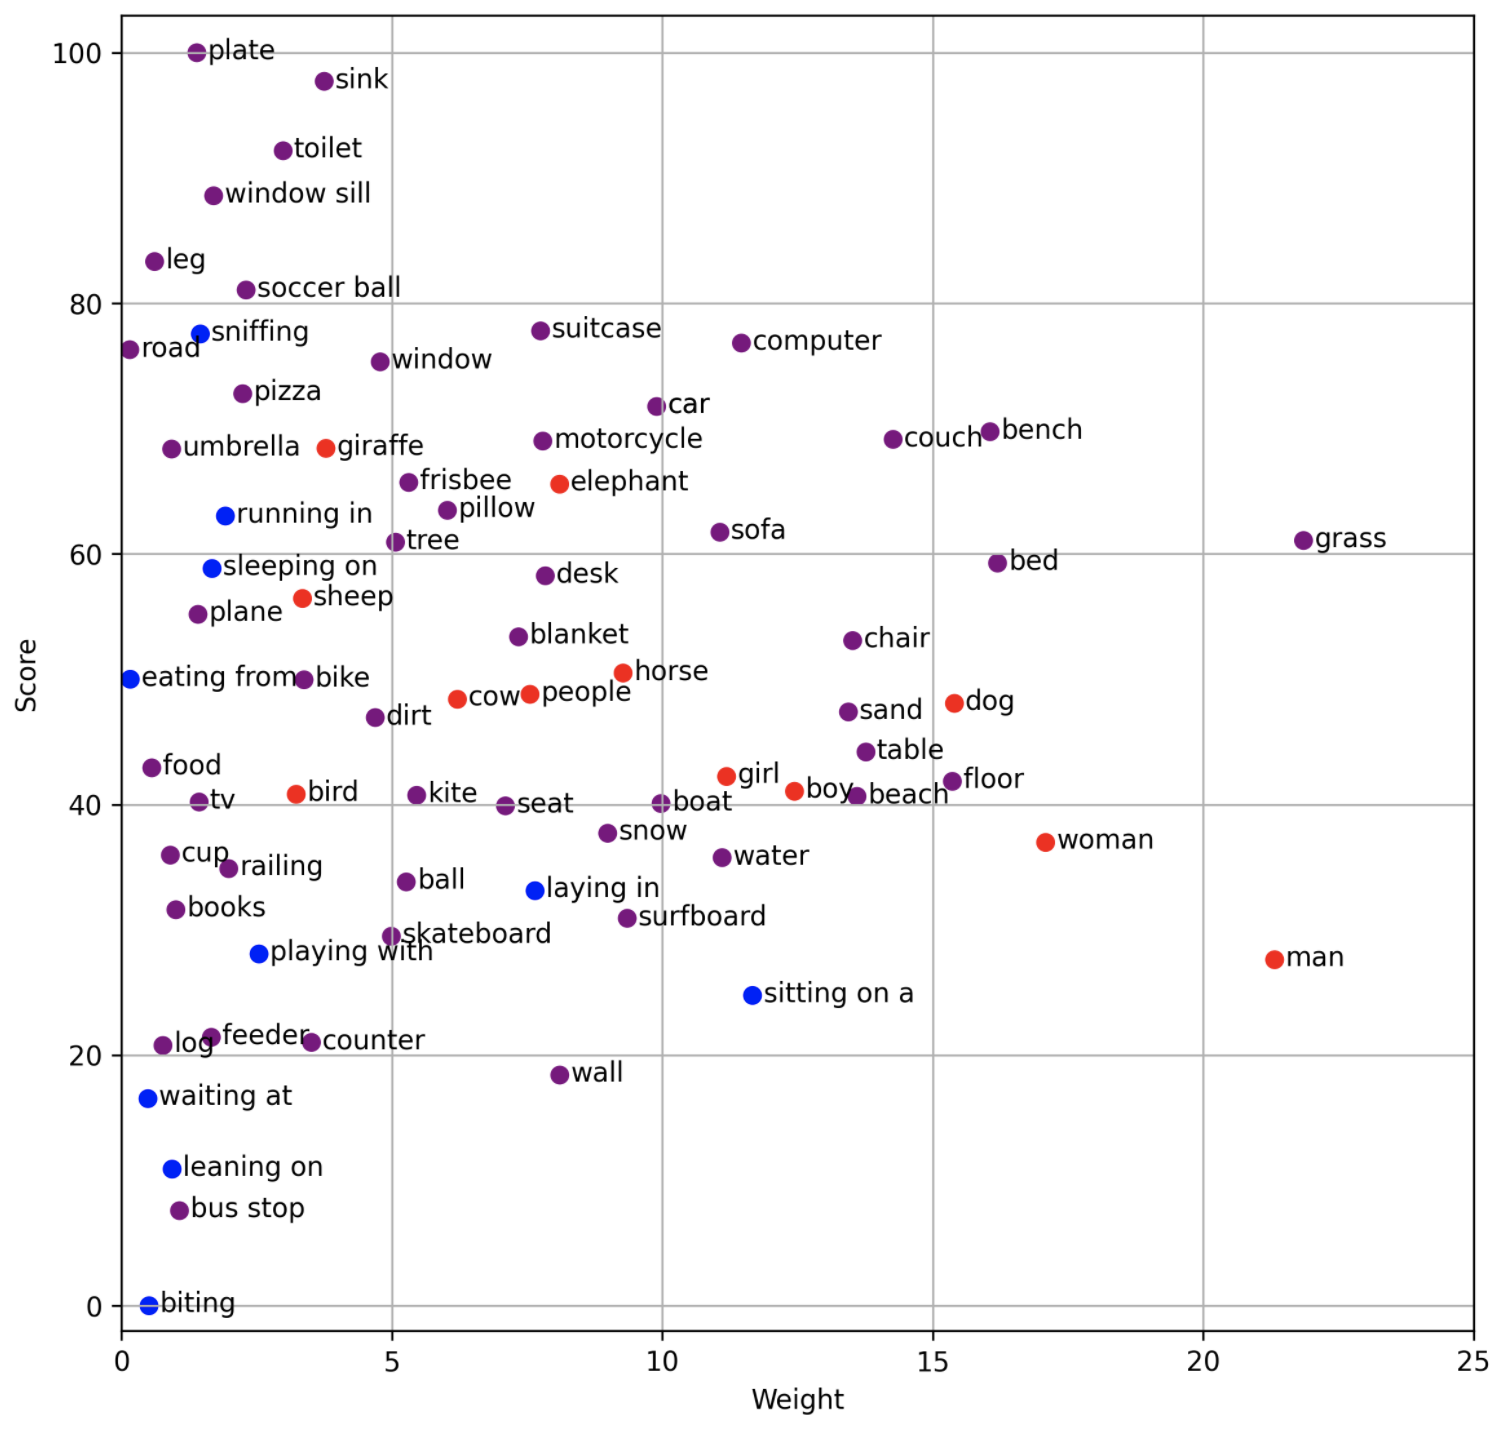}
    \caption{Score breakdown by target. Subjects are in red, relations in blue and objects are in purple. The model used is CLIP finetuned with $\tau=0.1$}
    \label{fig:breakdown}
\end{figure}

In Figure \ref{fig:breakdown}, we use the CLIP model finetuned with $\tau=0.1$ and compute the SIMAT score by grouping transformations by their target values: for each word $w$, we compute the weighted accuracy of transformation success for all queries $\wi$ such that $w_2 = w$. The relative weight of each target value in the final SIMAT score in shown on the x-axis, and the y-axis represents the SIMAT score. We can see that overall, transforming object relations is harder than transforming the objects themselves, which is probably because relationship are less easily identifiable in images. Also, if we compare the SIMAT scores between objects, we can see that the best SIMAT scores are obtained for objects that are easy to recognize (sink, toilet, suitcase..) while the worst scores correspond to objects without a well defined shape that are harder to recognize (feeder, counter, wall, bus stop).

\subsection{Validation on SIC112}

In this final section, we use the SIC112 dataset \cite{vo2019let} to validate our delta vector-based transformation method. As explained in Section~\ref{sec:data:eval}, the metric used is the accuracy of transformation success based on the original annotation of the retrieved image. They report a baseline accuracy of 26.6.
We highlight the most important results in Table~\ref{fig:sic}, where we use the same accuracy score and the same Image retrieval upper bound method as a point of comparison.

\begin{table}[H]
\centering
\small
\begin{tabular}{cccc}
\toprule
%\thead{Method} & \thead{SIC \\ Score} & \thead{Image retrieval \\ Upper Bound} \\
\MC{2}{c}{\thead{Method}} & \thead{SIC} & \thead{Image retrieval} \\[-3pt]
\thead{Image} & \thead{Text} & \thead{Score} & \thead{Upper Bound} \\
\midrule

\MC{2}{c}{Vo et al. \cite{vo2019let}} & 26.6 & 39.6 \\
\MC{2}{c}{CLIP zero shot} ($\lambda$=1)& 20.4 & 70.1 \\
\MC{2}{c}{CLIP zero shot} ($\lambda$=3) & 31.7 & 70.1 \\
CLIP & CLIP & 47.4 & 71.8 \\
CLIP & FastText & 50.7 & 53.3 \\
RN50 & FastText & 26.7 & 52.5 \\
\bottomrule
\end{tabular}
\caption{\label{fig:sic} Comparison of several algorithms for semantic image transformation on the SIC112 dataset.
%X + Y refers to the algorithm with image encoder X and text encoder Y.
}
\vspace{-10pt}
\end{table}

The zero-shot CLIP method reaches a lower score than the baseline with $\lambda=1$ but a higher score with $\lambda=3$, which is in accordance with our results on SIMAT. Fine-tuning with $\tau=0.1$ dramatically improves the SIC112 score (although not shown here, the scores for $\tau=0.01$ are lower). We also observe that using FastText embeddings yields even higher scores, although the Image retrieval Upper bound is much lower than that of the CLIP-only model.
Note that our method with Resnet50 reaches the same accuracy as \cite{vo2019let} while not being trained with a transformation objective.

Figure \ref{fig:sicenc} shows an ablation conducted on the image and text encoders used for transferring transformation on SIC112. Here, the choice of sentence embeddings has little influence while the CLIP image encoder outperforms its Resnet counterparts (45-50\% SIMAT score vs 25-30\%). This is probably because SIC112 images do not naturally belong to the image distribution of ImageNet or COCO, on which the Resnet are trained, whereas CLIP is trained on a much broader image distribution.

\begin{figure}
    \centering
    \includegraphics[width=0.9\linewidth]{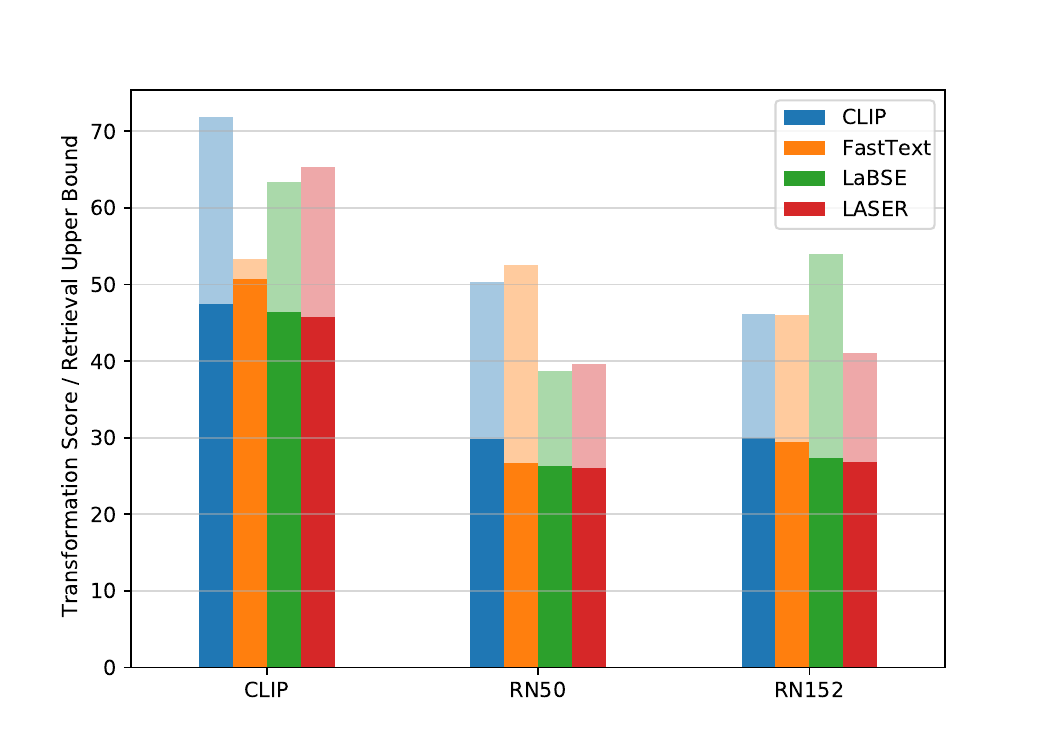}
    \caption{SIC score for multiple image/text encoders. Retrieval Upper bound is shown in transparency.}
    \label{fig:sicenc}
    \vspace{-10pt}
\end{figure}
